# Supplementary material for: Latent-Optimized Adversarial Neural Transfer for Sarcasm Detection
Source: arXiv:2104.09261 source file (2021-08-16)
Supplement: Supplementary file 1 [file appendix.tex]

\section{Appendix}
\label{sec:appendix}

\begin{equation*}
\begin{split}
\odv{\mathcal{L}^{'}}{\Phi_{sh}} &= \left( \odv{\mathcal{L}_s(z_s)}{\Phi_{sh}} + \odv{\mathcal{L}_s(z_s^{'})}{\Phi_{sh}} \right) + \left( \odv{\mathcal{L}_t(z_t)}{\Phi_{sh}} + \odv{\mathcal{L}_t(z_t^{'})}{\Phi_{sh}} \right) - \odv{\mathcal{L}_d(z_s, z_t)}{\Phi_{sh}} 
\end{split} 
\end{equation*}
Applying chain rule, we have
\begin{equation*}
\begin{split}
\odv{\mathcal{L}_s(z_s^{'})}{\Phi_{sh}}=\pdv{\mathcal{L}_s(z_s^{'})}{\Phi_{sh}} +  \pdv{\mathcal{L}_s(z_s^{'})}{z_s^{'}}\pdv{z_s^{'}}{\Phi_{sh}}=\pdv{\mathcal{L}_s(z_s^{'})}{\Phi_{sh}} + \pdv{\mathcal{L}_s(z_s^{'})}{z_s^{'}}\left(\pdv{z_s}{\Phi_{sh}} + \eta \pdv{\mathcal{L}_d^{2}(z_s)}{z_s\Phi_{sh}}\right)
\end{split} 
\end{equation*}
Similarly,
\begin{equation*}
\begin{split}
\odv{\mathcal{L}_t(z_t^{'})}{\Phi_{sh}}=\pdv{\mathcal{L}_t(z_t^{'})}{\Phi_{sh}} + \eta \pdv{\mathcal{L}_t(z_t^{'})}{z_t^{'}}\pdv{\mathcal{L}_d^{2}(z_t)}{z_t^{'}\Phi_{sh}}
\end{split} 
\end{equation*}
Thus
\begin{equation*}
\begin{split}
\odv{\mathcal{L}^{'}}{\Phi_{sh}} =\pdv{\mathcal{L}}{\Phi_{sh}} + \pdv{\mathcal{L}_s(z_s^{'})}{\Phi_{sh}} + \pdv{\mathcal{L}_t(z_t^{'})}{\Phi_{sh}} + \eta \pdv{\mathcal{L}_s(z_s^{'})}{z_s^{'}}\pdv{\mathcal{L}_d^{2}(z_s)}{z_s^{'}\Phi_{sh}} + \eta \pdv{\mathcal{L}_t(z_t^{'})}{z_t^{'}}\pdv{\mathcal{L}_d^{2}(z_t)}{z_t^{'}\Phi_{sh}}
\end{split} 
\end{equation*}
